# Supplementary material for: Anchor Data Augmentation
Source: arXiv:2311.06965 source file (2023-11-27)
Supplement: Supplementary file 1 [file appendix_only.tex]

\documentclass{article}
% if you need to pass options to natbib, use, e.g.:
%     \PassOptionsToPackage{numbers, compress}{natbib}
% before loading neurips_2020

% ready for submission
\usepackage{neurips_2023}
\usepackage{wrapfig}
% to compile a preprint version, e.g., for submission to arXiv, add add the
% [preprint] option:
%     \usepackage[preprint]{neurips_2020}

% to compile a camera-ready version, add the [final] option, e.g.:
%     \usepackage[final]{neurips_2020}

% to avoid loading the natbib package, add option nonatbib:
%     \usepackage[nonatbib]{neurips_2020}

\usepackage[utf8]{inputenc} % allow utf-8 input
\usepackage[T1]{fontenc}    % use 8-bit T1 fonts
\usepackage{hyperref}       % hyperlinks
\usepackage{url}            % simple URL typesetting
\usepackage{booktabs}       % professional-quality tables
\usepackage{amsfonts}       % blackboard math symbols
\usepackage{nicefrac}       % compact symbols for 1/2, etc.
\usepackage{microtype}      % microtypography

\usepackage{algorithm}
\usepackage{algorithmic}
\usepackage{float}
\usepackage{macros}
\usepackage{neurips_2023}

\usepackage[rightcaption]{sidecap}
\usepackage{graphicx}

\usepackage{natbib}
\includeonly{sec:}

% uncomment for last run
% \nofiles

\title{Anchor Data Augmentation}

% The \author macro works with any number of authors. There are two commands
% used to separate the names and addresses of multiple authors: \And and \AND.
%
% Using \And between authors leaves it to LaTeX to determine where to break the
% lines. Using \AND forces a line break at that point. So, if LaTeX puts 3 of 4
% authors names on the first line, and the last on the second line, try using
% \AND instead of \And before the third author name.

\author{%
  Nora Schneider\\
  Computer Science Department\\ ETH Zurich\\ Zurich, Switzerland\\
  \texttt{nschneide@student.ethz.ch} \\
  % examples of more authors
   \And
  Shirin Goshtasbpour \\
  Computer Science Department\\ ETH Zurich\\ Zurich, Switzerland\\
  \texttt{shirin.goshtasbpour@inf.ethz.ch} \\
   \AND
  Fernando Perez-Cruz \\
  Swiss Data Science Center\\ Zurich, Switzerland\\
  \texttt{fernando.perezcruz@sdsc.ethz.ch} \\
  % \And
  % Coauthor \\
  % Affiliation \\t
  % Address \\
  % \texttt{email} \\
  % \And
  % Coauthor \\
  % Affiliation \\
  % Address \\
  % \texttt{email} \\
}
% uncomment for last run
\nofiles
\input{preamble.tex}
\begin{document}
\appendix
\onecolumn
\input{sections/Appendix}
\end{document}
